# Supplementary material for: Minimal model of charge and pairing density waves in X-ray scattering experiments
Source: arXiv:1908.00566 source file (2020-07-02)
Supplement: Supplementary file 1 [file SupplementalMaterial.pdf]

# Supplementary Information

## A. THE MINIMIZATION PROCESS FOR t'/t

In this section, we show how to extract ratio $t'/t$ by minimizing the difference between $\chi(\mathbf{q}, \Omega = 0)$, Eqs. (3) and (4) and the experimental signal $I_{\rm exp}$. We realized this procedure by setting $\Delta_0/t$ to experimentally relevant values (see main text) and computing $\chi$ at 301 equally spaced $q$ points between $-\pi/a$ and $\pi/a$, which we denoted by $q_{\rm th}(j) = [(j-150)/150]\pi/a$, with $j = 0, 1, 2, ..., 300$. We then chose from this array the elements that were closest to the $n$ experimental points, $q_{\rm exp}(i)$ with $i = 1, ..., n$. We denoted these elements by $q_{th}(j_i)$ and defined $I_{\rm th}(i) = \chi(q_{\rm th}(j_i), \Omega = 0)$. Next, we spanned both the experimental and theoretical data from 0 to 1, by defining the normalized data

$$\tilde{I}_{\rm exp/th}(i) = \frac{I_{\rm exp/th}(i) - \min\{I_{\rm exp/th}\}}{\max[I_{\rm exp/th} - \min\{I_{\rm exp/th}\}]}. \tag{A.1}$$

Simply put, we subtracted the minimal value of the data and divided by the resulting maximum. We defined the root-mean-square of the difference between the theory and experiment:

$$\Delta I = \sqrt{\frac{1}{n}\sum_{i=1}^{n}\left[\tilde{I}_{\rm th}(i) - \tilde{I}_{\rm exp}(i)\right]^2}. \tag{A.2}$$

Finally, we minimized numerically $\Delta I$ with respect to $t'/t$. Fig. A1 shows such representative process for NCCO (Fig. 1(a) in the main text). For this material, we obtain a global minimum at $t'/t = -0.22$ for CDWs (blue) and $t'/t = -0.41$ for PDWs (red). We repeated the same process for the other two cuprates (Hg1201 and BSCCO) discussed in the main text. The resulting values of $t'/t$ are reported in the caption of Fig. 1 in the main text.

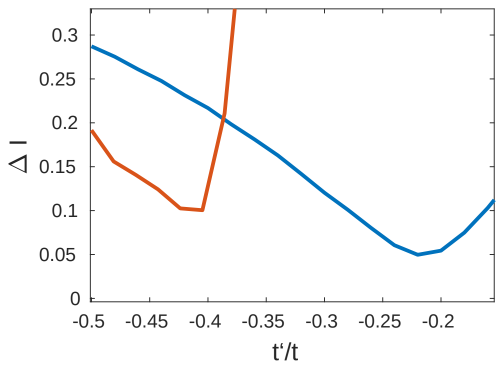


FIG. A1: The minimization process, Eq. (A.2) as a function of $t'/t$, for CDW (blue) and PDW (red).

## B. A HEURISTIC MODEL OF THE FERMI SURFACE FOR CDW AND PDW

In the main text, we gave a heuristic explanation why the CDW signal is peaked at $(\pm q, \pm q)$ while the PDW is peaked at $(\pm q, 0)$ and $(0, \pm q)$. This result can be better visualized by considering the simplified version of the Fermi surface of cuprates shown in Fig. B1(a). Due to the denominator in Eq. (3) (taking the static limit $\Omega = 0$), CDWs are mostly affected by $\mathbf{k}$ vectors such that $\varepsilon_{\mathbf{k}} \approx \varepsilon_{\mathbf{k}+\mathbf{q}} \approx 0$. Hence, this signal is naturally enhanced at nesting vectors $\mathbf{q}$ that connect parallel segments of the Fermi surface. In the Fermi surface of Fig. B1, the nesting condition is achieved at both $(q, 0)$ and $(q, q)$. As shown there, the segments of the Fermi surface contributing to the former (rectangles) are shorter than the segments contributing to the latter (rectangles and ellipses): their total lengths equal to, respectively, $2\pi/a - q$ and $4\pi/a - 4q$. Hence, for $q = 0.25 \times 2\pi/a$, this model predicts that $R = 3/4$, in quantitative agreement with the result obtain in the main text. In the case of the PDW signal, Eq. (4), each segment of the Fermi surface is weighted by the corresponding value of $\Delta_{\mathbf{k}}$. This factor strongly favors the wavevector $(q, 0)$, which connects antinodes to antinodes, with respect to $(q, q)$, which connects antinodes to nodes. Hence, for PDWs $R > 1$, as noted in the main text where we obtain $R = 1.4$ for PDW.

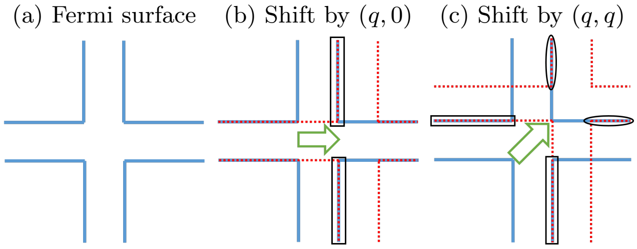


FIG. B1: (a) Simplified model of the Fermi surface of cuprates with well-defined nesting vectors. (b) Overlap between the Fermi surfaces $\varepsilon_{\mathbf{k}} = 0$ and $\epsilon_{\mathbf{k}+(q,0)} = 0$. The green arrow shows the direction of the shift towards the new Fermi surface (red dots). (c) Overlap between the Fermi surfaces $\varepsilon_{\mathbf{k}} = 0$ and $\varepsilon_{\mathbf{k}+(q,q)} = 0$. The black rectangles and ellipses indicate the segments of the Fermi surface that contribute to $\chi(\mathbf{q}, \Omega = 0)$ (see text).

## C. THE EFFECT OF DIFFERENT PINNING CENTERS

In the main text, we considered two types of pinning centers: A single site on which $U \to U + \delta U$ which acts as a charge impurity, and a single bond on which $V \to V + \delta V$, which corresponded to a pairing impurity. In the former case, we obtained a distinct peak in the $(q, q)$ direction, accompanied by mixed CDW/PDW fluctuations with $\delta\Delta/\delta n \approx 1$, whereas in the latter the signal peaked at $(q, 0)$ with dominant PDW fluctuations $\delta\Delta/\delta n \approx 140$. We concluded that the experimental signal observed in $(q, 0)$ is explained by PDW rather than CDW.

To demonstrate the robustness of this result, we consider here six additional pinning centers (see Fig. C1):

(a) $t \to t + \delta t$ on one bond, where $t$ is the NN hopping coefficient.

(b) $t' \to t' + \delta t'$ on one bond, where $t'$ is the NNN hopping coefficient.

(c) $t'' \neq 0$ on one bond, where $t''$ is the next-NNN hopping coefficient.

(d) $U \to U + \delta U$ on four adjacent nearest neighbors sites enclosing a square plaquette.

(e) $V \to V + \delta V$ on four adjacent nearest neighbors bonds enclosing a square plaquette.

(f) $V \to V + \delta V$ on four bond in a cross shape.

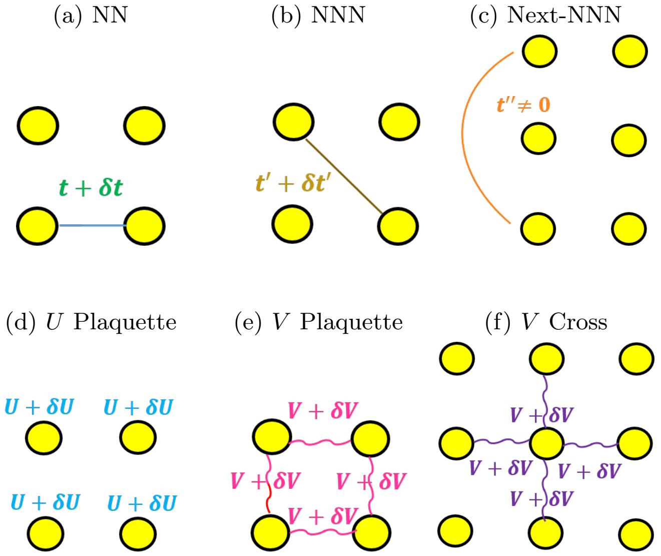


FIG. C1: Schematic picture of the different pinning centers considered in this Supplemental Material, embedded on a square lattice. The pinning center is given by the local modulation of: (a-c) The hopping coefficients $t$, $t'$, $t''$ on NN (green), NNN (gold) and next-NNN (orange) bonds, respectively. (d) The repulsive interaction $U$ on a plaquette (light blue). (e-f) The attractive interaction $V$ on a plaquette (pink), or four bonds in a cross shape (purple).

For each type of impurity, we self-consistently solved the mean-field equations of the extended Hubbard model. We find that the impurities (a-d) exhibit a clear peak in the $(q, q)$ direction, while (e-f) are peaked at $(q, 0)$, see Fig. C2. The corresponding values of $R \equiv \chi(\mathbf{q} = (q, 0), \Omega = 0)/\chi(\mathbf{q} = (q, q), \Omega = 0)$ and $\delta\Delta/\delta n$ are summarized in table I. We conclude that for the cases (a-d) the peaks are much stronger at $(q, q)$, i.e. $R < 1$, and there are mixed CDW/PDW

fluctuations such that $\delta\Delta/\delta n$ is of order 1. In contrast, the cases (e-f) have $R > 1$ and the fluctuations of the pairing gap $\delta\Delta$ are at least one order of magnitude larger than those of the density $\delta n$. These findings are analogous to the two examples reported in the main text and demonstrate their broad applicability.

| | $\delta U$ (main text) , | $\delta V$ (main text) | (a) | (b) | (c) | (d) | (e) | (f) |
|---|---|---|---|---|---|---|---|---|
| $R$ | 0.63 | 1.97 | 0.77 | 0.33 | 0.35 | 0.62 | 1.33 | 1.74 |
| $\delta\Delta/\delta n$ | 1.06 | 140 | 1.66 | 1.61 | 1.75 | 1.06 | 16 | 19 |

TABLE I: $R$-values and $\delta\Delta/\delta n$ for the different pinning centers. Note that all cases that resemble a charge impurity have $R < 1$ and $\delta\Delta/\delta n$ of order 1, while for those that resemble a pairing impurity $R > 1$ and $\delta\Delta$ is at least one order of magnitude grater than $\delta n$.

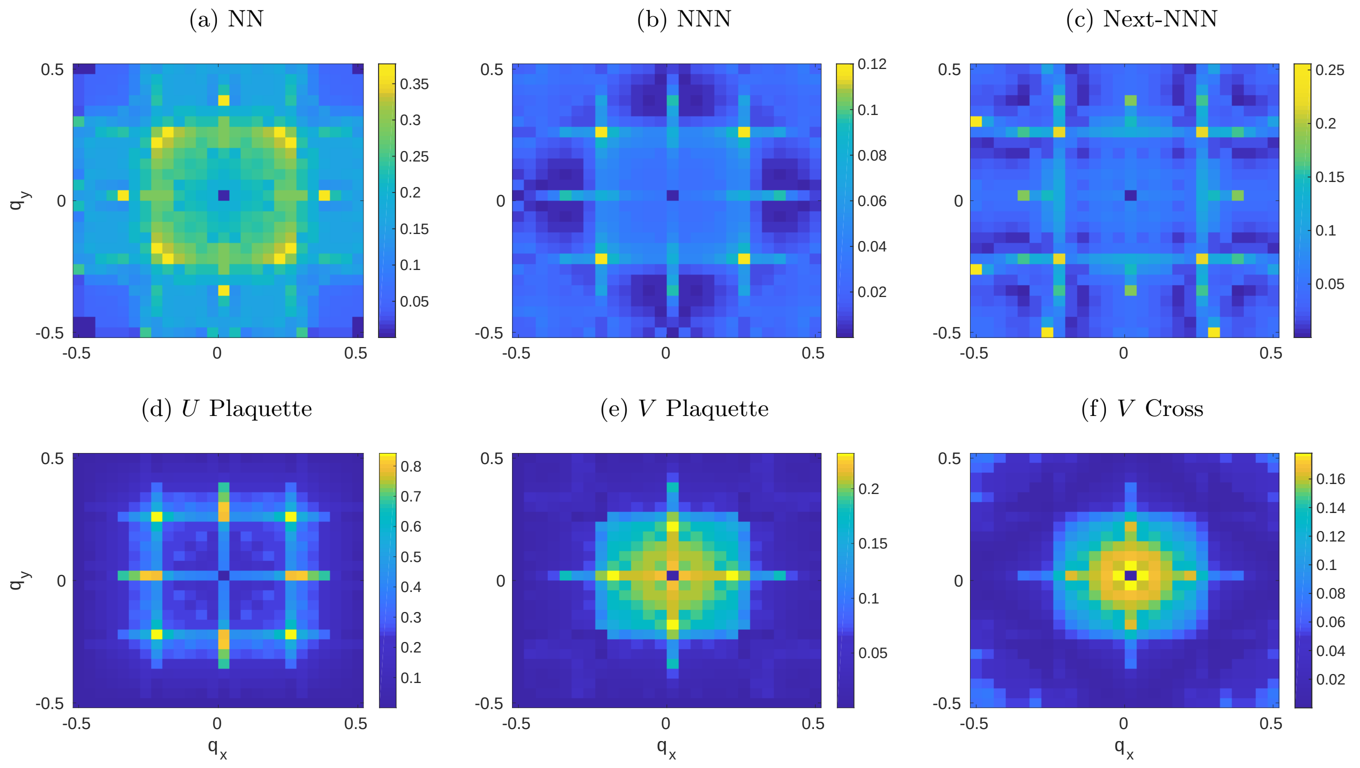


FIG. C2: Fourier transform of the density, $n_{\mathbf{q}}$, induced by the impurities described in Fig. C1. Subplots (a-d) are peaked at $(q, q)$, while (e-f) are peaked at $(q, 0)$, with $q/2\pi \approx 0.25$. The numerical values are $U/t = 1.5, V/t = -0.5, t'/t = -0.6, \delta U/t = \delta V/t = \delta t = \delta t'/t = 0.2$ and $t''/t = 0.2$ in (c).

## D. DOPING DEPENDENCE

In this section, we compare the theoretical and experimental dependence of the peak wavevector on the doping. According to our weak-coupling approach, the wavevector of the CDW/PDW peak is related to a nesting vector that connects parallel segments of the Fermi surface. As such, one expects that changing the doping will effect this vector, i.e. the signal will peaked at a different $\mathbf{q}$. In particular, as the doping of holes increases, the Fermi surface shrinks and, as a result, $\mathbf{q}$ decreases. This effect is demonstrated in Fig. D1, where we show the position of the PDW peak in Eq. (4) of the main text, as a function of doping. The observed dependence matches the experimental observations of Refs. [15, 24].

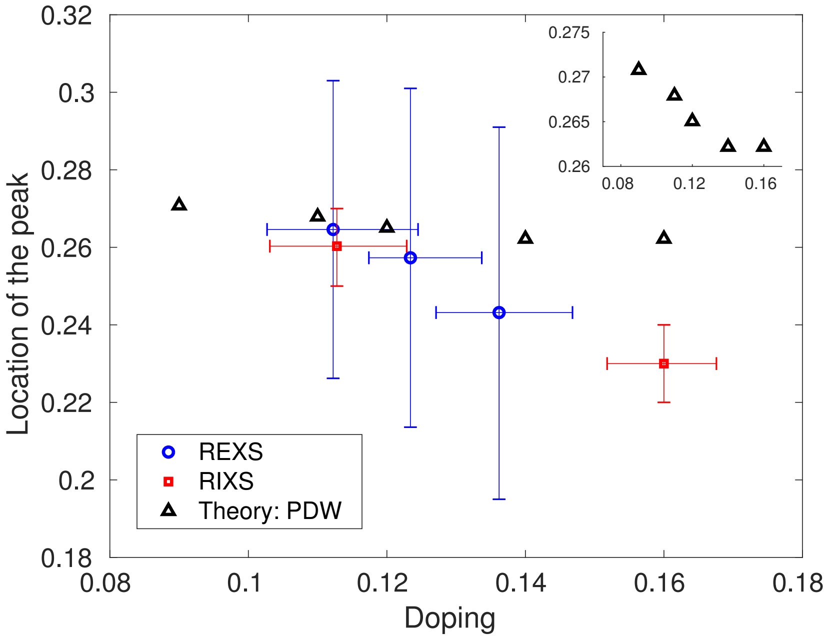


FIG. D1: Doping dependence of the PDW wavevector: Experimental results, reproduced from Ref. [14] (blue circles, REXS) and Ref. [24] (red squares, RIXS), along with their error bars. Theoretical prediction of the PDW signal, Eq. (4) of the main text, for different doping values (black triangles, see inset). The numerical values are the same as in Fig. 1 of the main text: $t'/t = -0.7,\ \Delta_0/t = 0.3$.
